# Supplementary material for: Distributed Signaling Games
Source: arXiv:1404.2861 source file (2015-07-05)
Supplement: Supplementary file 1 [file AppendixProofs.tex]

\newcommand{\reuniformdistributionsproof}
{
\begin{proof}
Let $d$ be the common denominator of $\mu(j)$ for every $j \in I$ (i.e., for every item $j \in I$, $d \cdot \mu(j)$ is an integer). Intuitively, we construct the new instance by splitting every item $j \in I$ into $d \cdot \mu(j)$ identical copies. Following is a formal construction.

Let $\tilde{n} = dn$, and let $\{\tilde{I}_j\}_{j \in I}$ be a partition of $[\tilde{n}]$ where $|\tilde{I}_j| = d \cdot \mu(j)$. The value of bidder $i$ for item $\tilde{j} \in [\tilde{n}]$ is $v_{i,j}$, where $j$ is the single item of $I$ for which $\tilde{j} \in \tilde{I}_j$. The function $\sigma$ is defined as following:
\[
	\sigma(\cP)
	=
	\{\cup_{j \in S} \tilde{I}_j ~\mid~ S \in \cP\}
	\enspace,
\]
and the partition of mediator $t \in M$ under the new model is $\tilde{\cP}_t = \sigma(\cP_t)$. It can be easily checked that a partition $\tilde{\cP}_t$ is a refinement of $\tilde{\cP}'_t$ if and only if there exists a partition $\cP'_t$ for which $\cP_t$ is a refinement and $\sigma(\cP'_t) = \tilde{\cP}'_t$. Next, fix a strategy profile $\cP'_1,\cP'_2, \ldots, \cP'_m$. Then:
\begin{align*}
	R(\cappart_{t = 1}^m \cP'_t)
	={} &
	\sum_{S \in \cappart_{t = 1}^m \cP'_t} \mu(S) \cdot \smax_{i \in B}(v_{i, S})
	=
	\sum_{S \in \cappart_{t = 1}^m \sigma(\cP'_t)} \frac{|S|}{d} \cdot \smax_{i \in B}(v_{i, S})\\
	={} &
	\sum_{S \in \cappart_{t = 1}^m \sigma(\cP'_t)} \tilde{\mu}(S) \cdot \smax_{i \in B}(v_{i, S})
	=
	R(\cappart_{t = 1}^m \sigma(\cP'_t))
	\enspace.
	\qedhere
\end{align*}
\end{proof}
}

\newcommand{\clcontinuesdominantproof}
{
\begin{proof}
We prove the statement for mediator $1$. Since the players' information sets are symmetric, an analogues argument follows for mediator $2$. Let $\p \subseteq \cP_1$ be a non-continuous strategy for player $1$. Let $\cN = \{S \in \p ~\mid~ \text{$S$ is not continuous}\}$ be the collection of sets in $\p$ that are non-continuous. We suggest the following strategy for mediator $1$:
\[
	\p'
	=
	(\p \setminus \cN) \cup \bigcup_{S \in \cN} \cC(S)
	\enspace.
\]

In the rest of the proof, we show that for every strategy $\cP_2' \subseteq \cP_2$ of player $2$, $\Pi_1(\p', \cP_2') - \Pi_1(\p, \cP_2') > 0$. By definition,
\begin{align}\label{eq_payoff_delta1}
	\Pi_1(\p',\cP_2') - \Pi_1(\p,\cP_2')  = \frac{1}{2} (R_{\p'} - R_{\p})+ \frac{1}{2} (R_{\p' \cappart 		\cP_2'} - R_{\p \cappart \cP_2'}) \enspace.
\end{align}

By the way the $\DSP_\cS(n, n, 2)$ instance was constructed, if $S'$ and $S''$ are two disjoint sets such that no element of $S$ is adjacent to an element of $S'$ (according to their order in $V$), then $|S' \cup S'| \cdot v(S' \cup S') = \max\{|S'| \cdot v(S'), |S''| \cdot v(S'')\} $. Let us lower bound the two terms on the right hand side of (\ref{eq_payoff_delta1}):
\begin{align*}
	R_{\p'} - R_{\p}
	={} &
	\sum_{S \in \cN} \left[\sum_{S' \in \cC(S)} \mu(S') \cdot v(S') - \mu(S) \cdot v(S) \right] \WWW{\\}
	= \WWW{{} &}
	\sum_{S \in \cN} \left[\sum_{S' \in \cC(S)} \frac{|S'| \cdot v(S')}{n} - \frac{|S| \cdot v(S)}{n} \right]\\
	={} &
	\sum_{S \in \cN} \left[\sum_{S' \in \cC(S)} \frac{|S'| \cdot v(S')}{n} - \max_{S' \in \cC(S)} \left\{\frac		{|S'| \cdot v(S')}{n}\right\} \right]
	>
	0
	\enspace,
\end{align*}
where the last inequality is strict because $\cN \neq \varnothing$ and $|\cC(S)| > 1$ for every $S \in \cN$. Similarly, for the second term on the right hand side of (\ref{eq_payoff_delta1}), we get:

\begin{align*}
	R_{\p' \cappart \cP_2'}& - R_{\p \cappart \cP_2'}
	=
	\sum_{S \in \cP_2'} \sum_{\substack{S' \in \cN \\ S \cap S' \neq \varnothing}} \left[\sum_			{\substack{S'' \in \cC(S') \\ S \cap S'' \neq \varnothing}} \mu(S \cap S'') \cdot v(S \cap S'') - \mu(S 	\cap S') \cdot v(S \cap S') \right]\\
	={} &
	\sum_{S \in \cP_2'} \sum_{\substack{S' \in \cN \\ S \cap S' \neq \varnothing}} \left[\sum_			{\substack{S'' \in \cC(S') \\ S \cap S'' \neq \varnothing}} \frac{|S \cap S''| \cdot v(S \cap S'')}{n} - 		\frac{|S \cap S'| \cdot v(S \cap S')}{n} \right]\\
	={} &
	\sum_{S \in \cP_2'} \sum_{\substack{S' \in \cN \\ S \cap S' \neq \varnothing}} \left[\sum_			{\substack{S'' \in \cC(S') \\ S \cap S'' \neq \varnothing}} \frac{|S \cap S''| \cdot v(S \cap S'')}{n} - 		\max_{\substack{S'' \in \cC(S') \\ S \cap S'' \neq \varnothing}} \frac{|S \cap S''| \cdot v(S \cap S'')}{n} \right]
	\geq
	0
	\enspace.
\end{align*}

Plugging both the last inequalities into (\ref{eq_payoff_delta1}) completes the proof of the claim.
\end{proof}
}

\newcommand{\clonlyfullequproof}
{
\begin{proof}
We prove the statement for mediator $1$. Since players information sets are symmetric, an anlogues argument follows for mediator $2$. We also assume $|\p|, |\cP_2'| > 1$. The cases where $|\p| = 1$ and/or $|\cP_2'| \ = 1$ will be dealt separately latter. By definition,
\begin{align}\label{eq_payoff_delta2}
\Pi_1(\cP_1,\cP_2') - \Pi_1(\p,\cP_2')  = \frac{1}{2} (R_{\cP_1} - R_{\p})+ \frac{1}{2} (R_{\cP_1 \cappart \cP_2'} - R_{\p \cappart \cP_2'}) \enspace.
\end{align}

Let us lower bounds the terms on the right hand side of (\ref{eq_payoff_delta2}).
\begin{align*}
	R_{\cP_1} - R_{\p}
	={} &
	\sum_{S \in \cP_1 \setminus \p} \mu(S) \cdot v(S) - \sum_{S \in \p \setminus \cP_1} \mu(S) \cdot 	v(S) \WWW{\\}
	=\WWW{{} &}
	\sum_{S \in \cP_1 \setminus \p} \frac{|S|}{n} \cdot \frac{1}{2} - \sum_{S \in \p \setminus \cP_1} 		\frac{|S|}{n} \cdot \frac{1 + \eps}{|S|} \\
	={} &
	\frac{|\cP_1 \setminus \p| - (1 + \eps) \cdot |\p \setminus \cP_1|}{n}
	=
	\frac{1}{2} + \frac{\eps \cdot |\cP_1 \cap \p| - (1+ \eps) \cdot |\p|}{n}
	\enspace.
\end{align*}

Given a set $S \in \cP_2'$, let $e(S, \p) = |\{S' \in \p ~|~ |S \cap S'| = 1\}|$. Intuitively, $e(S, \p)$ is the number of endpoints of $S$ that are left as singletons in $\p \cappart \cP_2'$. Notice that $e(S, \p) \in \{0, 1, 2\}$. Let us look at a set $S \in \cP_2'$, and observe what becomes of it in $\p \cappart\cP_2'$. Notice that either $S \in \p \cappart \cP_2'$, or $S$ is split into multiple sets in $S \in \p \cappart \cP_2'$, two of which contain the end elements of $S$, and are of odd size. The other sets resulting from $S$ are of even size, and therefore, are not singletons. The same observation also holds for $\cP_1 \cappart \cP_2'$, but here the odd sets must be singletons, and the even sets are of size exactly $2$. Finally, observe that $|\p \cappart \cP_2'| = |\p| + |\cP_2'|$. This is true since the (cyclically) leftmost element of every set in $\p \cappart \cP_2'$ must be the leftmost element of exactly one set in $\p$ or $\cP_2'$, and vice versa. Using these observations, we get:
{
\ArchiveX{\allowdisplaybreaks}
\begin{align*}
	R_{\cP_1 \cappart \cP_2'}& - R_{\p \cappart \cP_2'}
	=
	\sum_{S \in \cP_2'} \left[ \sum_{\substack{S' \in \cP_1 \setminus \p \\ S \cap S' \neq \varnothing}} 	\mu(S \cap S') \cdot v(S \cap S') - \sum_{\substack{S' \in \p \setminus \cP_1\\ S \cap S'		 	\neq \varnothing}} \mu(S \cap S') \cdot v(S \cap S') \right]\\
	\geq{} &
	\sum_{S \in \cP_2'} \left[ \sum_{\substack{S' \in \cP_1 \setminus \p \\ |S \cap S'| = 2}} \frac{2}{n}		\cdot \frac{1}{2} + \WWW{\mspace{-9mu}} \sum_{\substack{S' \in \cP_1 \setminus \p \\ |S \cap S'| = 1}}  \frac{1}{n} \cdot \eps - \WWW{\mspace{-9mu}} \sum_{\substack{S' \in \p \setminus \cP_1\\ |S \cap S'| > 1}} \frac{|S \cap S'|}{n} \cdot \frac{1 + \eps}{|S \cap S'|} - \WWW{\mspace{-9mu}} \sum_{\substack{S' \in \p \setminus \cP_1\\ |S \cap S'| = 1}} \frac{1}{n} \cdot \eps \right]\\
	={} &
	\sum_{S \in \cP_2'} \left[ \sum_{\substack{S' \in \cP_1 \setminus \p \\ |S \cap S'| = 2}} \frac{1}{n} 		- \sum_{\substack {S' \in \p \setminus \cP_1\\ |S \cap S'| > 1}} \frac{1 + \eps}{n} + (2 - e(S, \p)) 		\cdot \frac{\eps}{n} \right]\\
	={} &
	\sum_{S \in \cP_2'} \frac{|S|/2 - 1 - |\{S' \in \cP_1 \cap \p ~|~ S' \subseteq S\}|}{n} \\
	&- \frac{(1 + \eps) \cdot \left[|\p \cappart \cP_2'| - \sum_{S \in \cP_2'} e(S, \p) - \sum_{S \in 			\cP_2'} |\{S' \in \cP_1 \cap 	\p ~|~ S' \subseteq S\}| \right]}{n} \\
	&+ \sum_{S \in \cP_2'} (2 - e(S, \p)) \cdot \frac{\eps}{n}\\
	={} &
	\frac{1}{2} + \frac{(\eps - 2) \cdot |\cP_2'|}{n} + \sum_{S \in \cP_2'} \frac{\eps \cdot |\{S' \in \cP_1 		\cap \p ~|~ S' \subseteq S\}| + e(S, \p)}{n} - \frac{(1 + \eps) \cdot |\p|}{n}
	\enspace.
\end{align*}
}

Plugging the last two inequalities into (\ref{eq_payoff_delta2}) gives:
\begin{align*}
	2[\Pi_1(\cP_1,\cP_2') -& \Pi_1(\p,\cP_2')]
	\geq
	1 + \frac{\eps \cdot |\cP_1 \cap \p| - 2(1+ \eps) \cdot |\p| + (\eps - 2) \cdot |\cP_2'|}{n} \\
	&+ \sum_{S \in \cP_2'} \frac{\eps \cdot |\{S' \in \cP_1 \cap \p ~|~ S' \subseteq S\}| + e(S, \p)}{n}
	\enspace.
\end{align*}

Notice that $\sum_{S \in \cP_2'} e(s, P_1')$ is the number of singletons in $\p \cappart \cP_2'$. The other sets in $\p \cappart \cP_2'$ must be of size at least $2$. Moreover, the number of sets of size at most $2$ in $\p \cappart \cP_2'$ is upper bounded by $|\cP_2'| + |\cP_1 \cap \cP_1'|$ (each set of size $2$ in $\p \cappart \cP_2'$ originates from a set of either $\cP_2'$ or $\cP_1 \cap \cP_1'$ included in a set of the other partition, and every set of size of odd size originates from a pair of overlapping sets). Thus,
\begin{align*}
	&
	2|\p \cappart \cP_2'| + [|\p \cappart \cP_2'| - |\cP_2'| - |\cP_1 \cap \cP_1'|] - \sum_{S \in \cP_2'} e		(s, P_1') \leq n\\
	\Rightarrow{} &
	\sum_{S \in \cP_2'} e(s, P_1') \geq 3|\p \cappart \cP_2'| - |\cP_2'| - |\cP_1 \cap \cP_1'|] - n = 3|\p| 	+ 2|\cP_2'| - |\cP_1 \cap \cP_1'|] - n
	\enspace.
\end{align*}

Plugging the last inequality into the previous one gives:
\begin{align*}
	2[\Pi_1(\cP_1,\cP_2') - \Pi_1(\p,\cP_2')]
	\geq{} &
	\frac{(1 - 2\eps) \cdot |\p| - (1 - \eps) \cdot |\cP_1 \cap \p| + \eps \cdot |\cP_2'|}{n} \\
	&+ \sum_{S \in \cP_2'} \frac{\eps \cdot |\{S' \in \cP_1 \cap \p ~|~ S' \subseteq S\}|}{n}
	\enspace.
\end{align*}

Notice that for a set of $\cP_1 \cap \p$ to not be included in any set of $\cP_2'$, it must be on the border between two sets of $\cP_2'$. Therefore, the number of such sets is at most $|\cP_2|$. Therefore, $\sum_{S \in \cP_2'} |\{S' \in \cP_1 \cap \p ~|~ S' \subseteq S\}| + |\cP_2'| \geq |\cP_1 \cap \p|$. Plugging this into the previous inequality gives:
\[
	2[\Pi_1(\cP_1,\cP_2') - \Pi_1(\p,\cP_2')]
	\geq
	\frac{(1 - 2\eps) \cdot |\p| - (1 - 2\eps) \cdot |\cP_1 \cap \p|}{n}
	\enspace,
\]
and the right hand side of the last inequality must be strictly positive because if $\p \subseteq \cP_1$, then $\p = \cP_1$ because they are both partitions of $I$, which contradicts the conditions of the lemma. This completes the proof of the first case.

Next, consider the case where $|\cP_2'| = 1$. In this case,
\begin{align}\label{eq_payoff_delta3}
	\Pi_1(\cP_1,\cP_2') - \Pi_1(\p,\cP_2')  = R_{\cP_1} - R_{\p} \enspace.
\end{align}

We clearly have $R_{\cP_1} = 1/2$. Let $a$ and $b$ denote the number of sets in $R_{\p}$ of sizes $2$ and larger than $2$, respectively. Clearly, $2a + 4b \leq n$. Therefore,
\[
	R_{\p}
	=
	\sum_{S \in \p} \nu(S) \cdot v(S)
	=
	a \cdot \frac{2}{n} \cdot \frac{1}{2} + \sum_{\substack{S \in \p \\ |S| > 2}} \frac{|S|}{n} \cdot \frac{1 	+ \eps}{|S|}
	=
	\frac{a+ b(1 + \eps)}{n}
	<
	\frac{a+ 2b}{n}
	\leq
	\frac{1}{2}
	\enspace,
\]
where the inequality holds since $\eps < 1$ and $b \geq 1$. Plugging the last two observations into (\ref{eq_payoff_delta3}) completes the proofs of the case.

Finally, consider the case where $|\p| = 1$ but $|\cP_2'| > 1$. In this case:
\begin{align}\label{eq_payoff_delta4}
\Pi_1(\cP_1,\cP_2') - \Pi_1(\p,\cP_2')  = \frac{1}{2} (R_{\cP_1} - R_{\cP_1'}) + \frac{1}{2} (R_{\cP_1 \cappart \cP_2'} - R_{\cP_2'}) \enspace.
\end{align}

Again $R_{\cP_1} = 1/2$, and it can be easily checked that $R_{\cP_1} = (1 + \eps)/n$. Let us lower bound the second term of (\ref{eq_payoff_delta4}).
\begin{align*}
	R_{\cP_1 \cappart \cP_2'} -& R_{\cP_2'}
	=
	\sum_{S \in \cP_2'} \left[ \sum_{\substack{S' \in \cP_1 \\ S \cap S' \neq \varnothing}} \mu(S \cap 		S') \cdot v(S \cap S') - \mu(S) \cdot v(S) \right]\\
	\geq{} &
	\sum_{S \in \cP_2'} \left[ \sum_{\substack{S' \in \cP_1 \\ |S \cap S'| = 2}} \frac{2}{n} \cdot \frac{1}		{2} + \sum_{\substack{S' \in \cP_1 \\ |S \cap S'| = 1}}  \frac{1}{n}	\cdot \eps - \frac{|S|}{n} \cdot 		\frac{1 + \eps}{|S|} \right] \WWW{\\}
	= \WWW{{} &}
	\sum_{S \in \cP_2'} \left[ \sum_{\substack{S' \in \cP_1 \\ |S \cap S'| = 2}} \frac{1}{n} + \frac{2\eps}		{n} - \frac{1 + \eps}{n}  \right]\\
	={} &
	\sum_{S \in \cP_2'} \frac{|S|/2 - 2 + \eps}{n}
	=
	\frac{1}{2} + \frac{(\eps - 2) \cdot |\cP_2'|}{n}
	\geq
	\frac{1}{2} + \frac{(\eps - 2) \cdot (n/2)}{n}
	=
	\frac{\eps - 1}{2}
	\enspace.
\end{align*}

Plugging all the above inequalities into (\ref{eq_payoff_delta4}), we get:
\[
	2[\Pi_1(\cP_1,\cP_2') - \Pi_1(\p,\cP_2')]
	=
	\left[\frac{1}{2} - \frac{1 + \eps}{n}\right] + \frac{\eps - 1}{2}
	=
	\frac{\eps}{2} - \frac{1+\eps}{n}
	>
	0
	\enspace,
\]
where the inequality follows from the definition of $\eps$. This completes the proof of the last case.
\end{proof}
}

\newcommand{\legonepropertiesproof}
{
\begin{proof}
The instance $\cG_1$ we construct contains $2n^5$ equal probability items, $2n^5$ bidders and $n$ mediators. Bidder $i$ has a 
value of $2n^5$ for item $i$, and a value of $0$ for every other item (the valuations matrix of $\cG_1$ is depicted as Figure~\ref{fig:G_1_matrix}). The partition $\cP_t$ of every mediator $t$ is determined by a set 
$I_t \subseteq \{1, 2, \ldots, n^5\}$ as following. For every number $\ell \in I_t$, $\cP_t$ has two parts isolating items $2\ell - 1$ and $2\ell$, and for every number 
$\ell \not \in I_t$, $\cP_t$ has one part containing both $2\ell - 1$ and $2\ell$. More formally,
\[
	\cP_t = \{\{2\ell - 1\}, \{2\ell\} \mid \ell \in I_t\} \cup \{\{2\ell - 1, 2\ell\} \mid \ell \in \{1, 2, \ldots, n^5\} \setminus I_t\}
	\enspace.
\]

\begin{figure}[t]
$$ \cG_1: \;\;
\left(
\begin{matrix}
2n^5           &  0  & 0          & \ldots    & 0           & 0           &  0         \\
0           &  2n^5           & 0 & 0           & \ldots    & 0           &  0         \\
0           &    0           &  2n^5           & 0 & 0        & \ldots    &  0         \\
\vdots   & \vdots   & \vdots   & \ddots  & \vdots  & \vdots  & \vdots  \\
\vdots   & \vdots   & \vdots   & \vdots   & \ddots  & \vdots  & \vdots   \\
\vdots   & \vdots   & \vdots   & \vdots   & \vdots   & \ddots  & 0    \\
\eps  & 0            & 0   &\ldots   & \ldots            & 0            & 2n^5          \\
\end{matrix}
\right)
$$
\caption{The valuations matrix of the gadget $\cG_1$.} \label{fig:G_1_matrix}
\end{figure}

Observe that if no third party reports her partition, then the revenue of $\cG_1$ is $1$. Otherwise, if a non-empty set $T$ of third parties report their partitions, then 
$2\left|\bigcup_{t \in T} I_t\right|$ items become isolated, while the rest of the items are paired (recall that $\cG_1$ is an instance of the $\aon$ model). 
An isolated item has a zero contribution to the revenue (as the second highest price in every column of Figure~\ref{fig:G_1_matrix} is $0$), while a pair 
of item is selected with probability $2/(2n^5) = n^{-5}$ and has an expected value of $2n^5/2 = n^5$ for two bidders. Thus, each pair contributes exactly $1$ to the revenue. Since the number of pairs in $\cappart_{t \in T} \cP_t$ is $n^5 - \left|\bigcup_{t \in T} I_t\right|$, we get $R(\cappart_{t \in T} \cP_t) = n^5 - \left|\bigcup_{t \in T} I_t\right|$. We shall prove that it is possible to randomly choose sets $I_t$ that with high probability will obey the following properties.
\begin{itemize}
    \item For every set $T$ of $k$ mediators: $n^5 - \left|\bigcup_{t \in T} I_t\right| \geq 0.1 \cdot n^5$.
    \item For every set $T$ of at least $3k \cdot \ln n$ mediators: $n^5 - \left|\bigcup_{t \in T} I_t\right| \leq 5 n^2$.
\end{itemize}
Observe that the lemma follows immediately from the above properties and the discussion before them. Let $I_t$ be a random subset containing every element of $\{1, 2, \ldots, n^5\}$ with probability $1/k$, independently. Fix a set $T$ of $k$ mediators, and let $I_T = \bigcup_{t \in T} \cI_t$. An item of $\{1, 2, \ldots, n^5\}$ does not belong to $\cI_T$ with probability:
\[
    (1 - 1/k)^k
    \geq
    e^{-1} \cdot (1 - 1/k)
    \geq
    e^{-1}/2
    \enspace,
\]
where the last inequality holds for large enough $k$. Thus, the expected size of $\left|\bigcup_{t \in T} \cI_t\right|$ is at most $(1 - e^{-1} / 2) \cdot n^5 \leq 0.82 \cdot n^5$. Since items are selected into $I_T$ independently, we get, by the Chernoff bound, that:
\[
    \Pr\left[\left|\bigcup_{t \in T} \cI_t\right| \geq 0.9 n^5\right]
    \leq
    e^{-\frac{(0.9/0.82 - 1)^2 \cdot 0.9n^5}{3}}
    <
    e^{-2 \cdot 10^{-3} \cdot n^5}
    \enspace.
\]

Using the union bound, we get that the probability that there exists a set $T$ of $k$ third parties for which $\left|\bigcup_{t \in T} \cI_t\right| \geq 0.9 n^5$ is at most:
\[
    \binom{n}{k} \cdot e^{-2 \cdot 10^{-3} \cdot n^5}
    \leq
    n^k \cdot e^{-2 \cdot 10^{-3} \cdot n^5}
    =
    e^{k \ln n - 2 \cdot 10^{-3} \cdot n^5}
    \leq
    e^{n \ln n - 2 \cdot 10^{-3} \cdot n^5}
    \leq
    e^{-10^{-3} \cdot n^5}
    \enspace,
\]
where the last inequality holds for large enough $n$. Next, fix a set $T$ of $3k \cdot \ln n$ or more third parties. An item of $\{1, 2, \ldots, n^5\}$ does not belong to $I_T$ with probability:
\[
    (1 - 1/k)^{|T|}
    \leq
    (1 - 1/k)^{3k \cdot \ln n}
    \leq
    e^{-3 \ln n}
    =
    \frac{1}{n^3}
    \enspace.
\]

Thus, the expected size of $n^5 - \left|\bigcup_{t \in T} \cI_t\right|$ is at most $(1/n^3) \cdot n^5 = n^2$. %Let $R$ be a random set containing every item of 
%$\{1, 2, \ldots, n^5\}$, independently, with probability $1/n^2$. Since the items are selected into $\left|\bigcup_{t \in T} \cI_t\right|$ independently, we may 
%couple the random variables to guarantee:
%\[
%    \{1, 2, \ldots, n^5\} \setminus \bigcup_{t \in T} \cI_t \subseteq R \enspace.
%\]
Applying the Chernoff bound again we get:
\[
    \Pr\left[n^5 - \left|\bigcup_{t \in T} \cI_t\right| \geq 5n^2\right]
    \leq
    2^{-4n^2}
    \enspace.
\]
By the union bound, the probability that there exists a set $T$ of $3k \log n$ or more third parties for which $n^5 - 
\left|\bigcup_{t \in T} \cI_t\right| \geq 5n^2$ is at most:
\[
    2^n \cdot 2^{-4n^2}
    =
    2^{n - 4n^2}
    \leq
    2^{-3n^2}
    \enspace.
\]
Applying the union bound once more, we get that $\cG_1$ has both the above properties with high probability, which completes the proof of the lemma.
\end{proof}
}

\newcommand{\thapproximationpositive}
{
\begin{proof}
First, let us explain why one may assume $|I \setminus \cup_{t \in M} I_t| \leq 1$. Otherwise, let $I' = I \setminus \cup_{t \in M} I_t$. We replace all the items of $I'$ with a new item $j'$ having the following properties: $\mu(j') = \mu(I')$ and for every bidder $i \in B$, $v_{i j'} = v_{i, I'}$. It is easy to see that the new instance is equivalent to the original one since the items of $I'$ are not separated by $\cP_t$ for any $t \in M$.

By the above assumption, $\cappart_{t \in M} \cP_t = \{\{j\} \mid j \in I\}$. Furthermore, for every partition $\cP \in \Omega(I)$, there exists (and is easy to find) a strategy profile $(\cP'_1, \cP'_2, \ldots, \cP'_m)$ for which $\cP = \cappart_{t \in M} \cP'_t$. Thus, the problem of optimizing the revenue for our {\DSP} instance is equivalent to the problem studied by \cite{GNS07}. The theorem now follows from the $1/2$-approximation proved by \cite{GNS07} for their model.
\end{proof}
}

\newcommand{\thmpoaubtwoproof}
{
%\begin{proof}
Let $\cP' = (\cP'_1, \cP'_2, \ldots, \cP'_m)$ be an arbitrary strategy profile of the instance in question. The revenue of $\cP'$ is:\begin{align*}
		R(\cappart_{t = 1}^m \cP'_t)
		={} &
    \sum_{S \in \cappart_{t = 1}^m \cP'_t} \mspace{-9mu} \mu(S) \cdot v(S)
		\ArchiveX{=
		\sum_{S \in \cappart_{t = 1}^m \cP'_t} \mspace{-9mu} \mu(S) \cdot \left(\smax_{i \in B} \frac{\sum_{j \in S} \mu(j) \cdot v_{i,j}}{\mu(S)} 
			\right)}\\
		={} &
		\sum_{S \in \cappart_{t = 1}^m \cP'_t} \left(\smax_{i \in B} \sum_{j \in S} \mu(j) \cdot v_{i,j}\right)
    \enspace.
\end{align*}

For every bidder $i \in B$, let $\Sigma_i = \sum_{j \in I} \mu(j) \cdot v_{ij}$. It is easy to see that $v(I) = \smax_{i \in B} \Sigma_i$ (in other words, the second highest $\Sigma_i$ value is $v(I)$). Let $i^* \in B$ be the index maximizing $\Sigma_{i^*}$ (breaking ties arbitrary). Consider a set $S \in \cappart_{t = 1}^m \cP'_t$. The elements of $S$ contribute at least $\smax_{i \in B} \sum_{j \in S} \mu(j) \cdot v_{i,j}$ to at least two of the values: $\Sigma_1, \ldots, \Sigma_n$. Thus, they contribute at least the same quantity to the sum $\sum_{i \in B \setminus \{i^*\}} \Sigma_i$. This means that at least one of the values $\{\Sigma_i\}_{i \in B \setminus \{i^*\}}$ must be at least:
\[
	\frac{\sum_{S \in \cappart_{t = 1}^m \cP'_t} \left(\smax_{i \in B} \sum_{j \in S} \mu(j) \cdot v_{i, j}\right)}{k - 1}
	=
	\frac{R(\cappart_{t = 1}^m \cP'_t)}{k - 1} \enspace.
\]
By definition $\Sigma_{i^*}$ must also be at least that large, and therefore, \[R(\{I\}) = v(I) \geq R(\cappart_{t = 1}^m \cP'_t) / (k - 1). \qedhere\]
%The theorem now follows from Theorem~\ref{th:better_then_silence} since $\cP'$ might be the optimal strategy profile.
%\end{proof}
}
